# Supplementary material for: PCFEx: Point Cloud Feature Extraction for Graph Neural Networks
Source: arXiv:2603.08540 source file (2026-03-09)
Supplement: Supplementary file 1 [file supplimental.tex]

\documentclass[lettersize,journal]{IEEEtran}
\usepackage{amsmath,amsfonts}
\usepackage{algorithmic}
\usepackage{array}
\usepackage[caption=false,font=normalsize,labelfont=sf,textfont=sf]{subfig}
\usepackage{textcomp}
\usepackage{stfloats}
\usepackage{url}
\usepackage{verbatim}
\usepackage{graphicx}
\usepackage{subfiles}
\usepackage{adjustbox}
\usepackage{multirow}
\usepackage{multicol}
\usepackage{caption}
\usepackage{makecell}
\usepackage{xcolor}
\usepackage{booktabs}
\usepackage{tabularx}
\usepackage[flushleft]{threeparttable}
\usepackage{hyperref}
% \hyphenation{op-tical net-works semi-conduc-tor IEEE-Xplore}
\def\BibTeX{{\rm B\kern-.05em{\sc i\kern-.025em b}\kern-.08em
    T\kern-.1667em\lower.7ex\hbox{E}\kern-.125emX}}
\usepackage{balance}
\begin{document}

\title{PCFEx: Point Cloud Feature Extraction for Graph Neural Networks (supplemental materials)}
\maketitle

\section{Result visualization for HPE}
In this section, we will share some visualization example of our prediction human pose estimation against the ground truth labels. We will show randomly sampled outputs for the validation/test dataset which were used for model evaluation. We will show some good examples along with some bad examples as much as possible. The 

\begin{figure}[h]
\centering\includegraphics[width=.48\textwidth]{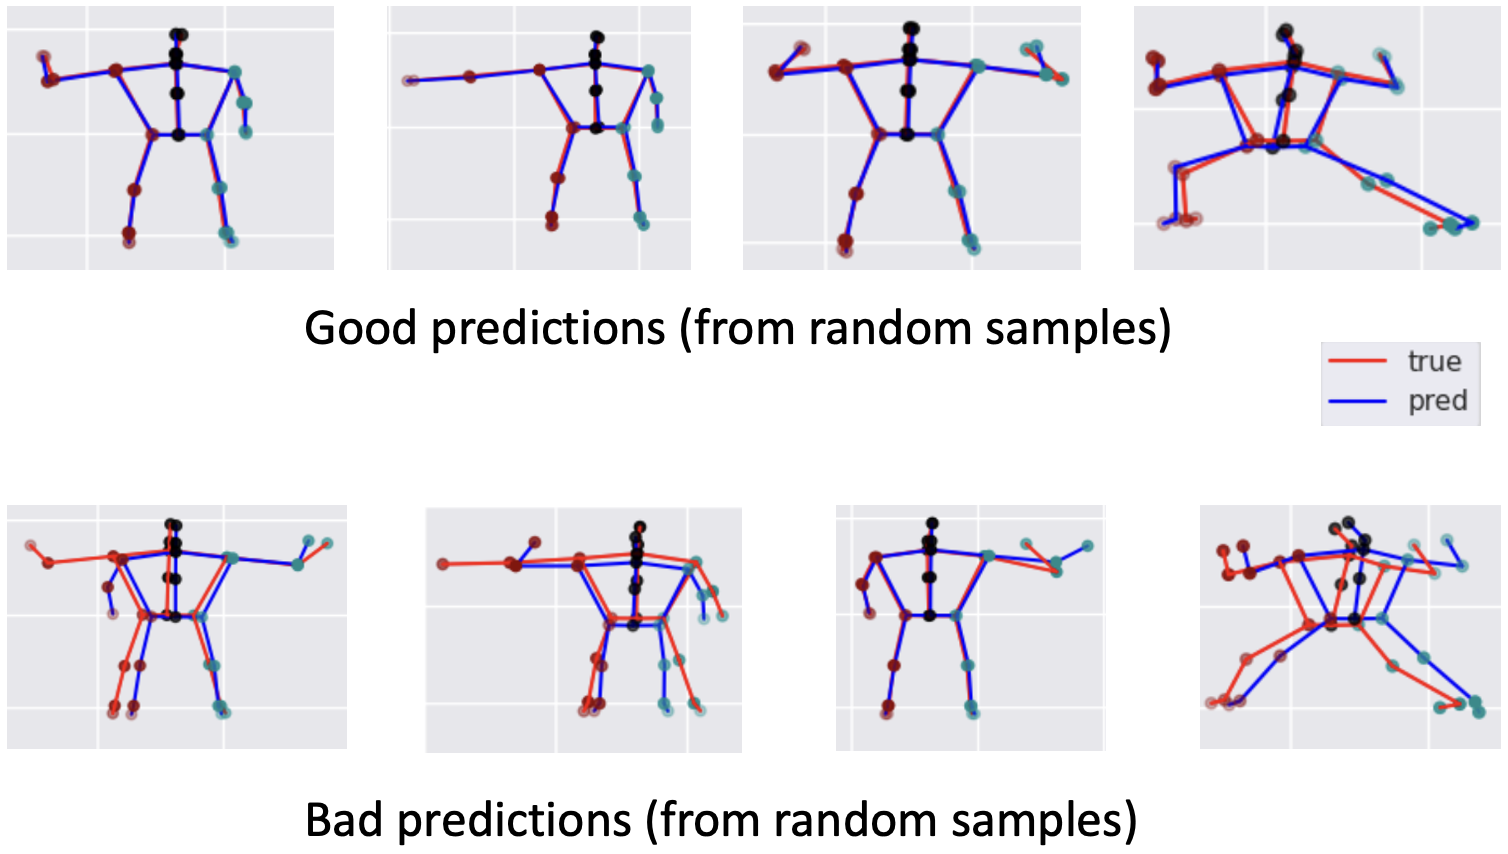}
\caption{Samples from MARS \cite{mars} test dataset.}
\label{mars-samples}
\end{figure}
From random samples, we selected some good and bad predictions by manually checking them. The model works comparatively better on MARS dataset samples leading to very small difference between the prediction and ground truth skeletons.

\begin{figure}[h]
\centering\includegraphics[width=.48\textwidth]{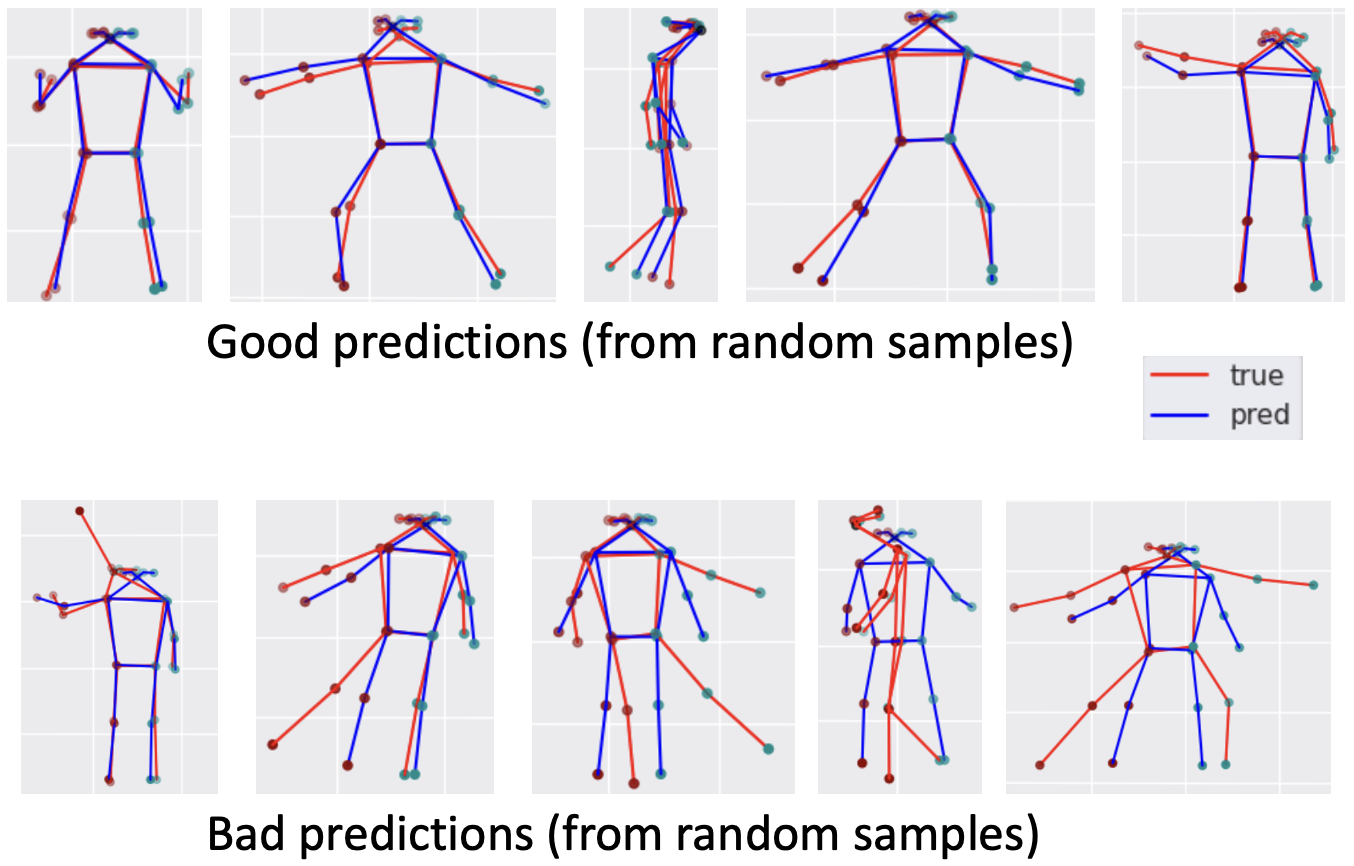}
\caption{Samples from mRI \cite{mri} validation set for the S2-P1 split.}
\label{mri-samples}
\end{figure}
mRI dataset are more diverse than MARS dataset in terms of number of activities, number of subjects etc. So, the predictions are not always so accurate, leading to comparatively higher difference between skeletons.

\begin{figure}[h]
\centering\includegraphics[width=.48\textwidth]{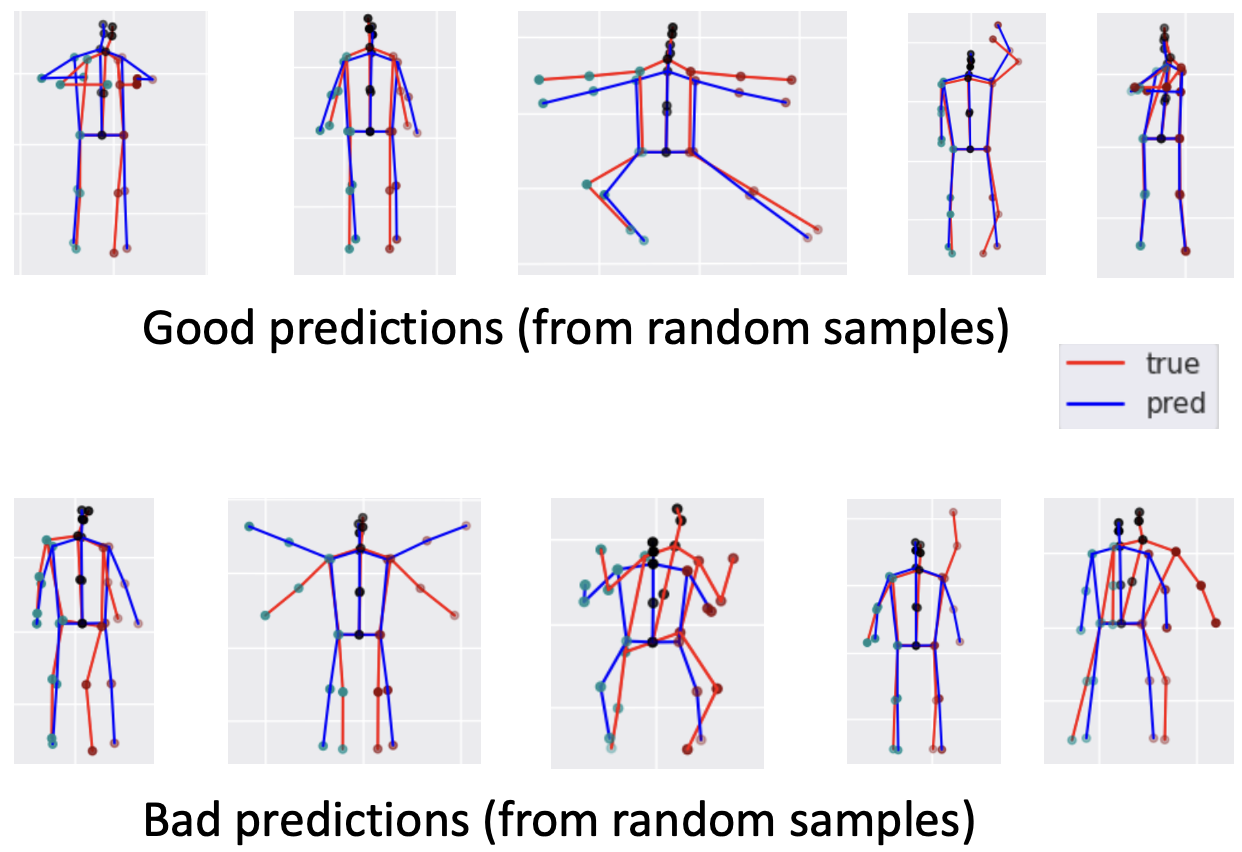}
\caption{Samples from MMFi \cite{mmfi} validation dataset for the S2-P3 split.}
\label{mmfi-samples}
\end{figure}
MMFi dataset is the most diverse dataset in terms of number of activities, number of subjects, using four different environments etc. Yet, our approach gets lower error on MMFi dataset than mRI dataset.
\begin{figure}[h]
\centering\includegraphics[width=.48\textwidth]{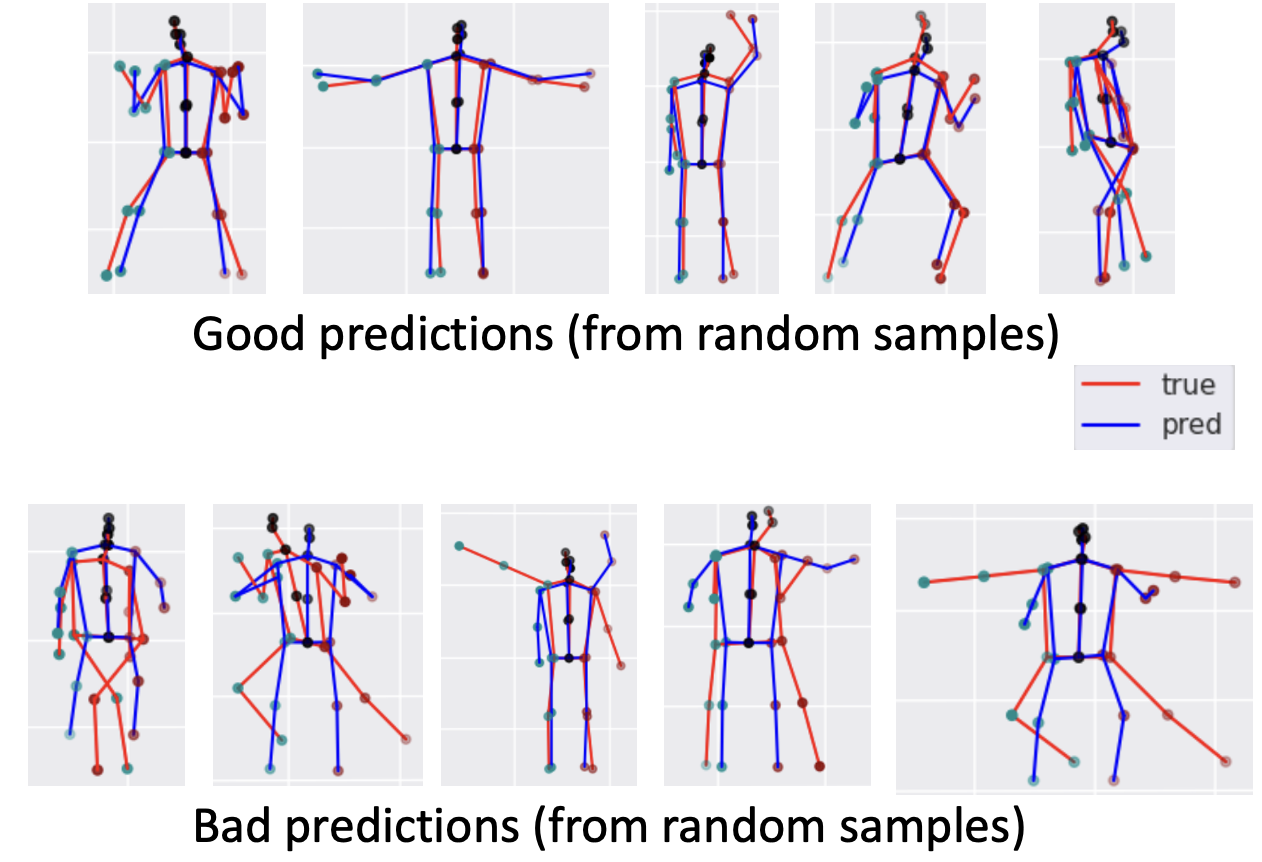}
\caption{Samples from MMFi \cite{mmfi} validation dataset for the S3-P3 split.}
\label{mmfi-samples-s3p3}
\end{figure}
Our assumption is that the data quality is better from their used sensor \cite{iwr-mmfi} than the sensor \cite{iwr1443boost} used by mRI and MARS datasets. Also, the data quality might be impacted by the high frequency setting of 30Hz in MMFi dataset than the low sampling rate of 10 Hz in mRI and MARS datasets. The Field of View is also larger in the IWR6483AOP sensor with 120$^{\circ}$ azimuth range and 120$^{\circ}$ elevation range. We didnt find specific azimuth and elevation range for the IWR1443BOOST module anywhere.

As described in the result comparison in \textit{Table \ref{mmfi-results}}, the skeleton predictions in S3-P3 (split by environment) are worse than S2-P3 (split by subjects). The sensor data acquisition is affected more by different environments and surroundings.

\begin{figure}[h]
\centering\includegraphics[width=.48\textwidth]{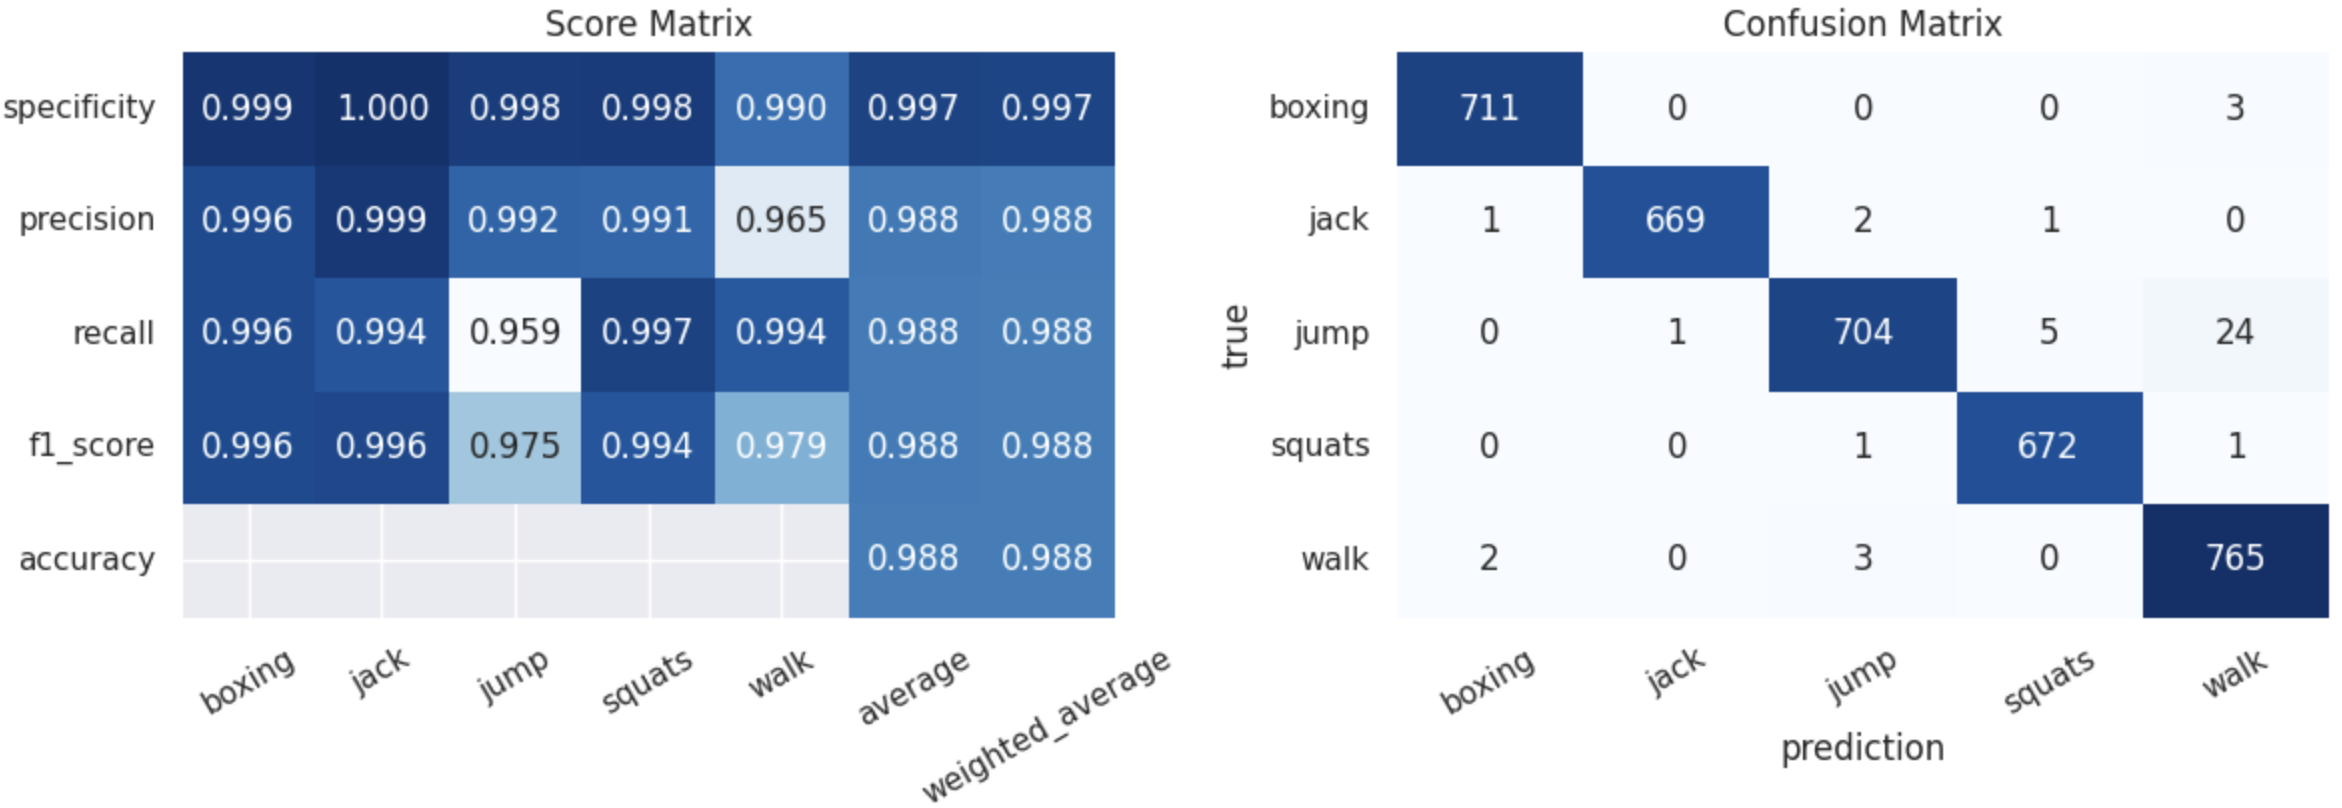}
\caption{Evaluation tables on the MMActivity \cite{radhar} test dataset}
\label{radhar-results-full}
\end{figure}
\begin{figure}[h]
\centering\includegraphics[width=.48\textwidth]{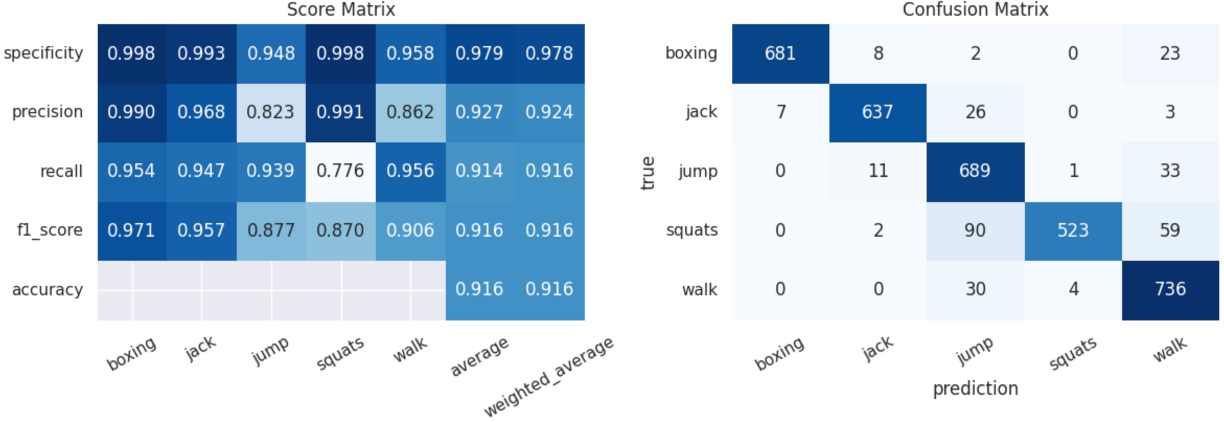}
\caption{Evaluation tables on the MMActivity \cite{radhar} test dataset without using the node and frame features}
\label{radhar-results-without}
\end{figure}
We show the complete result evaluation metrics on MMActivity dataset \cite{radhar} in \textit{Figure \ref{radhar-results-full}} for our approach. We also show the full result table on MMActivity dataset without using node and edge features in \textit{Figure \ref{radhar-results-without}}.

The complete results with pretrained models are uploaded \href{https://drive.google.com/drive/folders/1qqgeE9p96CsqV8g5--KZD6KeSktQ8l4a?usp=drive_link}{in this location}. All the samples shown above are collected from this location.

\section{Sequence Breaks for MARS dataset}
The MARS \cite{mars} dataset is provided in their \href{https://github.com/SizheAn/MARS}{Github repository} and they uploaded their used feature map data found in \href{https://github.com/SizheAn/MARS/tree/main/feature}{this location} which we used for our experimentation. The data actually had separate sequences but they accumulated all the sequences and put the whole data in tensors for each of train, validation and test sets. That's why for sequential modeling, we need to know the sequence breaking frames which we manually visualized and identified. The sequence break file shows the index of the first frame of each sequence. We uploaded the file \href{https://drive.google.com/file/d/15IVdeI8jW_KAS-kqrDE61a4LMnTTyJei/view?usp=sharing}{in this location}.

\section{Output results and model weight files}
We have uploaded our results on all five datasets in \href{https://drive.google.com/drive/folders/1RnYEHNhRg0LRgrE22U6hnv0uSRaOFKeR?usp=sharing}{this location}. There are two types of results found in our shared result directories. One is for regression type results, another is classification type results. The description to the result directories are given below-

\subsection{regression}
Inside the output directory for regression problems, we should see below things:
\begin{enumerate}
    \item runs directory: contains tensorboard files/checkpoints to check training progress using tensorboard
    \item cfg.yml: Contains config parameters for this execution
    \item learning-curves.png: Figure for the train and validation loss curves generated at the end of all epochs of the training
    \item loss-curves.csv, loss-curves.png: contains instant loss curve information after each epoch
    \item model-parameters.csv: shows number of trainable parameters of the ML model
    \item model-structure.txt: contains detailed architecture of the ML model
    \item model weight (.pt) files: model weight files are stored in .pt format. Best weight file is named as 'pytorch-best-model.pt'. 'pytorch-model.pt' is the weight file stored after the last epoch of the training.
    \item store-data.pickle: this file contains the predicted pose keypoints for all datasets
    \item Three directories (Train, Validation, Test) contain random ground truth and prediction samples for train, val and test sets
    \item mae-rmse-results csv files for train, val and test: This csv file contains individual average mae and rmse errors for different keypoints. Reported MAE, RMSE for MARS dataset are collected from here.
    \item results.csv: this file containing evaluation metrics for three datasets (train, validation, test) for different evaluation metrics such as MPJPE, PA-MPJPE, RMSE, MAE, R-square, PCK etc. Reported MPJPE and PA-MPJPE errors are collected from here.
    \item label vs prediction scatter plots: Three figures are stored showing the true label vs predicted value in a scatter plot
\end{enumerate}

\subsection{classification}
\begin{enumerate}
    \item runs directory: contains tensorboard files/checkpoints to check training progress using tensorboard
    \item cfg.yml: Contains config parameters for this execution
    \item learning-curves.png: Figure for the train and validation loss curves generated at the end of all epochs of the training
    \item loss-curves.csv, loss-curves.png: contains instant loss curve information after each epoch
    \item model-parameters.csv: shows number of trainable parameters of the ML model
    \item model-structure.txt: contains detailed architecture of the ML model
    \item model weight (.pt) files: model weight files are stored in .pt format. Best weight file is named as 'pytorch-best-model.pt'. 'pytorch-model.pt' is the weight file stored after the last epoch of the training.
    \item store-data.pickle: this file contains the predicted values for all datasets
    \item results.csv: contains average scores of specificity, precision, recall, f1-score for all classes, along with accuracy and weighted accuracy (weighted by class samples) for Train, Validation and Test datasets. Reported accuracy is collected from here.
    \item classification result figures for Train, Validation and Test: each figure contains
    \begin{enumerate}
        \item Score table: showing detailed evaluation metrics across all class labels for specificity, precision, recall, f1-score, accuracy. Reported results are collected from these figures.
        \item Confusion matrix: Shows the number of true and false predicted cases for all class labels
    \end{enumerate}
\end{enumerate}

\section{Impact Statement}
Our work for HPE and HAR from mmWave radar data has immense potential to create great impact in healthcare sector for remote patient monitoring, rehabilitation support for patient and elderly people, activity recognition, remote training support without violating privacy of people's daily lives, even in dark environments. In this work, we did not acquire any data by ourselves, used publicly available datasets where the researchers upheld all ethical aspects and regulations well with appropriate consents from the subjects participated in the experiment.

There might be concerns related to the applications of our HPE and HAR methods, but we strongly believe that due to the usage of mmWave data, the concern of violating privacy is timid. It is one of our goals to build safe and secure environment by utilizing the recent advancements in Machine Learning and sensitive data resources.

\bibliographystyle{IEEEtran}
\bibliography{ref.bib}
\end{document}
